# Supplementary material for: Atomic Scale Interfacial Transport at an Extended Evaporating Meniscus
Source: arXiv:1805.12560 ancillary file (2018-12-06)
Supplement: Supplementary file 1 [file Supplementary_Material.pdf]

Supplementary Material for

# Atomic Scale Interfacial Transport at an Extended Evaporating Meniscus

Yigit Akkus[a,b], Anil Koklu[a], Ali Beskok[a]

[a]Lyle School of Engineering, Southern Methodist University, Dallas, TX 75205, USA
[b]ASELSAN Inc., 06172 Yenimahalle, Ankara, Turkey

S1. Molecular dynamics simulations

S2. Modeling strategy

S3. Interface detection

S4. Mass flow through adsorbed region

S5. Uncertainty analysis

S6. Kinetic limit of evaporation

S7. Location and profile of evaporating meniscus for different heating loads

S8. Physical effects of periodic boundary conditions

S9. Evaporation area selection

S10. Supplementary Video

## S1. Molecular dynamics simulations

Two systems are simulated. Except the number of fluid (Ar) atoms and the interaction between fluid and solid atoms, both systems are identical and subjected to same computational procedure. Systems have identical channel walls composed of (3240x2=6480) Platinum (Pt) atoms. Each wall has 4 solid layers and (1,0,0) crystal planes facing the liquid. The outermost layer of the walls is always fixed at their lattice positions. 4200 and 5775 fluid atoms are used in the first and second simulations, respectively. Numbers of fluid atoms are selected such that condensed phase is always attached to the channel inlets and outlets and the effective radius of curvature (based on a circular fit) at the interface is approximately the same for both systems, when the systems are isothermally equilibrated before the initiation of the heating/cooling process. Periodic boundary conditions are applied in all directions. Time step is 5 fs and each collected data is averaged for 2 ns. Lennard-Jones (L-J) 6-12 potential is used to model the interactions between Ar-Ar and Ar-Pt atoms with molecular diameters of $\sigma_{Ar}$ = 0.34 nm, $\sigma_{Ar\text{-}Pt}$ = 0.3085 nm, and depth of the potential wells of $\varepsilon_{Ar}$ = 0.01042 eV, $\varepsilon_{Ar\text{-}Pt}$ = 0.00558 eV for the first and $\varepsilon_{Ar\text{-}Pt}$ = 0.0558 for the second simulation [S. Maruyama and T. Kimura, *Therm. Sci. Eng.* **7** (1999)]. L-J potential is truncated with a cut-off distance of $3\sigma_{Ar}$. Embedded atom model is utilized for Pt-Pt atomic interactions [25]. Simulations are started from the Maxwell-Boltzmann velocity distribution for all atoms at 110 K. Nosé-Hoover thermostat is applied to all atoms (except the outermost Pt layers) for 15 ns to stabilize the system temperature at 110 K. Then, microcanonical ensemble is applied to Ar atoms for 15 ns to equilibrate the system, while solid atoms are still subjected to the thermostat. At the end of the isothermal stage, stable liquid/vapor Ar mixture is attained at 110 K. Then, equal energy injection/extraction (first simulation: $\dot{q}$=11 nW, second simulation: $\dot{q}$=20 nW) is applied to the wall atoms located at the heating/cooling zones for 40 ns. Other wall atoms are not allowed to vibrate in order to eliminate heat conduction through the solid wall. During heating/cooling, fluid atoms are subjected to microcanonical ensemble. At the end of heating/cooling period, statistically stable phase changing liquid/vapor interfaces are formed at both ends of the channel. The rates of the steady passive liquid flow from condensing interface to evaporating interface through the channel are calculated as ‘728.7±20.3 $\#_{Ar}$/ns’ and ‘504.4±12.1 $\#_{Ar}$/ns’ for the first and second simulations, respectively. As an experimental observation [21,22], molecular layering of fluid near a solid should be considered as a link to the real-world behavior of the system. During all simulations, molecular layering of Ar is verified in the proximity of the walls. Moreover, the distribution and magnitude of the density peaks are in good agreement with the results of [S. Maruyama and T. Kimura, *Therm. Sci. Eng.* **7** (1999)], where same L-J potential parameters were used. All simulations are carried out using Large-scale Atomic/Molecular Massively Parallel Simulator (LAMMPS) [S. Plimpton, *J. Comput. Phys.* **117** (1995)].

## S2. Modeling strategy

A saturated liquid/vapor mixture has equal evaporation and condensation rates at the interface. To disturb the equilibrium, a pressure difference between the bulk vapor and the vapor just above the interface must be generated. In an enclosed system, evaporation can be favored by reducing the bulk vapor pressure or increasing the interface pressure. The first method can be applied by

continuously removing the vapor phase from the system. If the mixture is composed of water and air, controlling of relative humidity is an example of this procedure as it was performed by the recent experiments [12,13]. However, application of this methodology is not practical for MD modeling. Due to the computational cost of MD simulations, only a limited number of atoms/molecules can be simulated within restricted time spans. Continuous removal of atoms/molecules would decrease the total number of fluid atoms during a simulation. Before the establishment of a steady evaporation, fluid atoms can be totally consumed or drop below a certain amount, for which statistical averaging will not yield trustable results. In addition, as a deterministic simulation method MD preserves the number of simulated atoms. Therefore, instead of a transient process, a steady-state process, which preserves the total number atoms/molecules, is more reliable. To realize this, we use the recently proposed phase change induced pumping mechanism [20]. At the evaporator part of this pump, a stable evaporating liquid/vapor interface forms. Continuous heating at this part increases the temperature at the interface. Consequently, evaporation is sustained by the increase of interface pressure instead of removing vapor atoms/molecules. Selection of fluid type is also critical. The number of vapor atoms in the gas phase should be large enough for accurate statistical averaging. Therefore, the selected liquid should have high vapor pressure. Water, which was used in the recent experiments [12,13], is not a good choice for MD simulations due to its relatively low volatility. For instance, saturated water mixture in equilibrium at room temperature has the ratio of 1/50,000 vapor to total water molecules, which is unfavorable for MD simulations conducted in nano-scale volumes. Therefore, our modeling strategy aims to construct steady-state evaporation of a high volatile liquid in order to realize a statistically reliable evaporation analysis.

## S3. Interface detection

In order to determine the liquid/vapor interface, simulation domain is divided into rectangular bins and average fluid density is calculated at each bin. Starting from the outer gas phase region, density of each bin is checked in longitudinal directions and the first bins, where the bin density exceeds the cut-off density, are marked as the liquid/vapor interface. Cut-off density is selected slightly higher than the density of the first minimum density peak in the liquid phase, which is approximately 23% and 21% of the average bulk liquid density within the channel for the first and second simulations, respectively. Selection of a higher cutoff density implies the existence of a non-physical vapor region within the bulk liquid, which prevents detection of a continuous liquid/vapor interface. However, selection of a lower cutoff density results in a larger liquid volume and thicker adsorbed layers, which does not affect proper prediction of the mobility of adsorbed layers. Moreover, it is worth mentioning that calculation of evaporation rate is independent of the interface selection in our computational setup due to the steady evaporation and associated steady passive liquid flow within the channel. Rate of evaporation is estimated by calculating the mass flow rate from the liquid state at the mid-channel in each simulation.

## S4. Mass flow through adsorbed region

Mass flow rate through a cross section area, $A$, is functions of density, $\rho$, and velocity, $\vec{u}$ :

$$\dot{m} = \int (\rho\vec{u}) \cdot \vec{n}\, dA \tag{1}$$

where $\vec{n}$ is the unit normal vector of the surface, across which the mass flow is calculated. Within the adsorbed layer, mass flow rate along the surface coordinate '$s$' can be expressed per unit channel depth as follows:

$$\dot{m}'|_s = \int_0^{\delta^*} (\rho\vec{u}) \cdot \vec{n}\, d\delta \tag{2}$$

where $\delta$ is the coordinate along the surface normal and $\delta^*$ is the thickness of the adsorbed layer. Mass flow rate at a specific '$s$' location can be calculated by approximating the above equation using rectangle rule of numerical integration, which requires summing the mass flow rates through the bins positioned at this '$s$' location (see Figure S1).

$$\dot{m}'|_s = \left( b \sum_i (\rho\vec{u})_i \right) \cdot \vec{n} \tag{3}$$

where $b$ is the height of each bin. When the velocity vector ($\vec{u} = u\vec{\imath} + v\vec{\jmath}$) and the unit normal vector ($\vec{n} = n_x\vec{\imath} + n_y\vec{\jmath}$) are decomposed to its components in horizontal and vertical directions, equation (3) can be expressed in terms of the contributions of mass flow rate in the horizontal and vertical directions as follows:

$$\dot{m}'|_s = b \sum_i \left[ (\rho u)_i n_x + (\rho v)_i n_y \right] \tag{4}$$

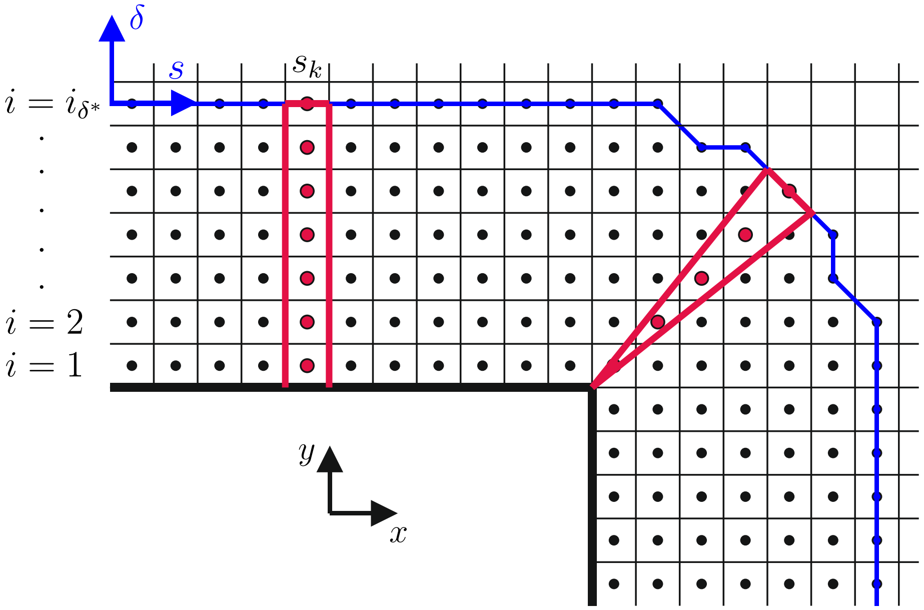


**Figure S1:** Mass flow calculation through adsorbed region. The figure is plotted for demonstration purposes and it does not reflect the real adsorbed layers observed in simulations, which contain much higher number

of bins. The dots show the center of each bin, where the flow properties are averaged in time. Blue line shows the liquid/vapor interface, which is formed by connecting the center of bins having higher density than the cut-off density (see Supplemental Material 3). Mass flow is calculated along this interface, i.e. along the surface coordinate '$s$'. Step size (arc length of interface at each step) is determined by connecting the mid points of two successive bin centers. Mass flow rate at each step is calculated by summing the mass flow rates of all bins located between the surface and wall. The red rectangle and the red dots within this region show contributing bins to the mass flow calculated at a certain step along the inner wall surface. The red triangle, on the other hand, specifies the contributing bins at a certain step at the corner region.

## S5. Uncertainty analysis

Density, velocities and temperature are sampled at every 2 ns and all the data collected between the two measurements is averaged, which yields a measurement uncertainty, $\varepsilon$, for each time averaged data, $\langle..\rangle$.

$$\rho = \langle \rho \rangle \pm \varepsilon_\rho \tag{5a}$$

$$u = \langle u \rangle \pm \varepsilon_u \tag{5b}$$

$$v = \langle v \rangle \pm \varepsilon_v \tag{5c}$$

$$T = \langle T \rangle \pm \varepsilon_T \tag{5d}$$

Uncertainties associated with density ($\varepsilon_\rho$), horizontal velocity ($\varepsilon_u$), vertical velocity ($\varepsilon_v$) and temperature ($\varepsilon_T$) are estimated by calculating the standard error of measurements, which is evaluated by dividing the standard deviation of measurements to the number of samples.

Mass flux is simply the multiplication of density and velocity. Estimation of mass flux has also associated uncertainty due to the time averaging.

$$\rho u = \langle \rho u \rangle \pm \varepsilon_{\rho u} \tag{6a}$$

$$\rho v = \langle \rho v \rangle \pm \varepsilon_{\rho v} \tag{6b}$$

Uncertainties of mass fluxes in horizontal and vertical directions are expressed in terms of the uncertainties of density and velocities as follows:

$$\varepsilon_{\rho u} = \sqrt{\left(\varepsilon_\rho u\right)^2 + (\varepsilon_u \rho)^2} \tag{7a}$$

$$\varepsilon_{\rho v} = \sqrt{\left(\varepsilon_\rho v\right)^2 + (\varepsilon_v \rho)^2} \tag{7b}$$

Mass flow rate through surface coordinate '$s$' is calculated using equation (4), where the mass flow rate under a specific surface coordinate '$s$' is the summation of horizontal and vertical mass fluxes through each bin positioned at the '$s$' location. Therefore, uncertainty of the mass flow rate depends on the uncertainties of mass fluxes at the contributing bins as shown in equation (8).

$$\dot{m}'|_s = b\left\langle \sum_i \left[(\rho u)_i n_x + (\rho v)_i n_y\right] \right\rangle \pm b\sqrt{\sum_i \left[\left(\varepsilon_{\rho u}\right)_i n_x\right]^2 + \left[\left(\varepsilon_{\rho v}\right)_i n_y\right]^2} \tag{8}$$

When equation (7) is inserted into equation (8), mass flow rate and its uncertainty can be expressed as the functions of the measured data and their measurement uncertainties as follows:

$$\dot{m}'|_s = b\left\langle \sum_i \left[(\rho u)_i n_x + (\rho v)_i n_y\right] \right\rangle \pm b\sqrt{\sum_i \left[\left(\varepsilon_\rho u\right)_i^{\,2} + (\varepsilon_u \rho)_i^{\,2}\right](n_x)^2 + \left[\left(\varepsilon_\rho v\right)_i^{\,2} + (\varepsilon_v \rho)_i^{\,2}\right]\left(n_y\right)^2} \tag{9}$$

## S6. Kinetic limit of evaporation

Hertz was the first to put an upper bound for the evaporation rates using kinetic theory of gases [9]. Later, Knudsen [10] derived the theoretical maximum rate of evaporation of a liquid into its own vapor in terms of intensive thermodynamic properties.

$$\dot{m}'' = \left(\frac{M}{2\pi R}\right)^{0.5}\left(\sigma_e \frac{p_{v,lv}}{\sqrt{T_{lv}}} - \sigma_c \frac{p_v}{\sqrt{T_v}}\right) \tag{10}$$

where $M$, $R$, $T_{lv}$, $p_{v,lv}$, $T_v$, $p_v$, $\sigma_e$, and $\sigma_c$ are molecular weight, universal gas constant, liquid/vapor interface temperature, vapor pressure just above the interface, vapor temperature, vapor pressure, evaporation coefficient and condensation coefficient, respectively. This equation is known as Hertz-Knudsen (H-K) equation, also known as the Hertz-Knudsen-Langmuir relation, and widely used to predict the kinetic limit of evaporation flux at the liquid-vapor interface.

A common approach is to take evaporation and condensation coefficients unity in the calculation of kinetic limit of evaporation. We first evaluated the kinetic limit with unit coefficients. Vapor pressure and temperature are measured away from the interface to capture the bulk properties of vapor. Interface temperature is calculated by averaging the temperature of the bins located at the interface. Interface pressure is taken as the equilibrium pressure of the vapor/liquid coexistence at the interface temperature.

Secondly, we evaluated the kinetic limit of evaporation based on the predictions of quantum-mechanically based statistical rate theory (SRT), which predicts the coefficients as follows [37]:

$$\sigma_e = \frac{p_{v,lv}}{p_v}\exp\left[(\mathrm{DOF}+4)\left(1 - \frac{T_v}{T_l}\right)\right]\left(\frac{T_v}{T_l}\right)^{\mathrm{DOF}+4} \tag{11a}$$

$$\sigma_c = \left(\frac{T_v}{T_l}\right)^{0.5}\exp\left[-(\mathrm{DOF}+4)\left(1 - \frac{T_v}{T_l}\right)\right]\left(\frac{T_l}{T_v}\right)^{\mathrm{DOF}+4} \tag{11b}$$

where, DOF is the vibrational frequency degrees of freedom, and three translational degree of freedom is predicted for an ideal monatomic gas [T.L. Hill, *An Introduction to Statistical Thermodynamics*; **Chapter 9,** Dover: Mineola, NY, (1986)]. The resultant coefficients were 2.17 and 0.98 for evaporation and condensation, respectively.

## S7. Location and profile of evaporating meniscus for different heating loads

Before heating, the system was isothermal and already equilibrated. Number of fluid atoms is selected such that liquid is attached to the channel inlets prior to heating. During simulations, different heating rates ($\dot{q}$) are applied to observe the response of evaporating meniscus. As shown in Figure S2, heating rates above 6 nW yield apparent meniscus deformations. Between 6 nW and 9 nW, evaporative mass flux increases more than 50% in the expense of a 10 K superheat rise. However, after 10 nW, mass flux slightly increases, whereas the superheat elevates more than 10 K. To explain this behavior, morphology of the liquid/vapor interface is examined at the each heating rate. Between 6 nW and 9 nW, liquid meniscus was attached to the channel inlets. However, after 10 nW, the extended meniscus is detached from the channel tips and receded into channel. During the simulation with 12 nW heating, evaporation resistance experienced a jump, which is accepted as the indication of burnout and the simulation is ceased. Second order curve fittings (red dashed curves) applied to these data groups and two different regimes (pinning and receding) are identified. This regime shift were previously demonstrated by a recent study [23], where the minimum nanopore modeled had a hydraulic dimeter of 20 nm.

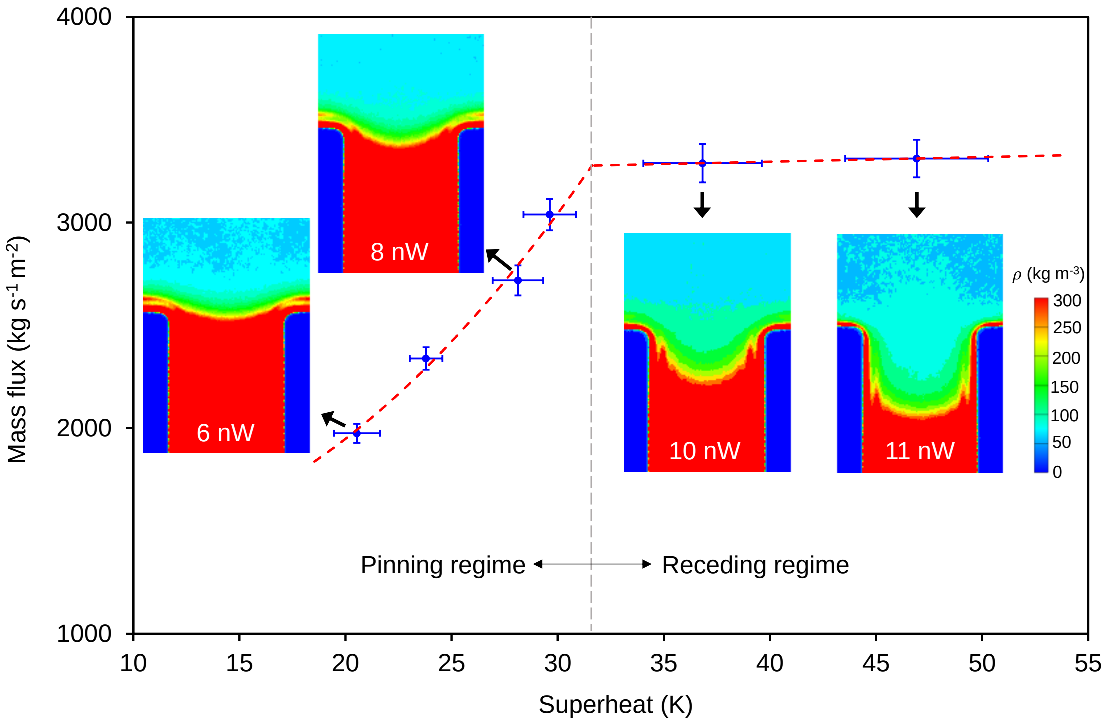


**Figure S2:** Evaporative mass flux vs. superheat for the first simulation together with the location and profile of evaporating meniscus at different heating rates.

## S8. Physical effects of periodic boundary conditions

We used periodic boundary conditions (PBCs) at all boundaries of the simulation domain. Using PBCs has advantages such as eliminating the surface effects and keeping the same number of molecules within the simulation domain. On the other hand, application of PBCs in all directions is geometrically equivalent to replication of the simulation domain throughout the space to form an infinite lattice (see Figure S3). For the sake of brevity, we included only the neighbor images to a sample simulation domain in the figure. The center plane of each wall is actually a stagnation zone due to the merging of two opposite streams. This stagnation plane and the opposing streams are emphasized in the close up view.

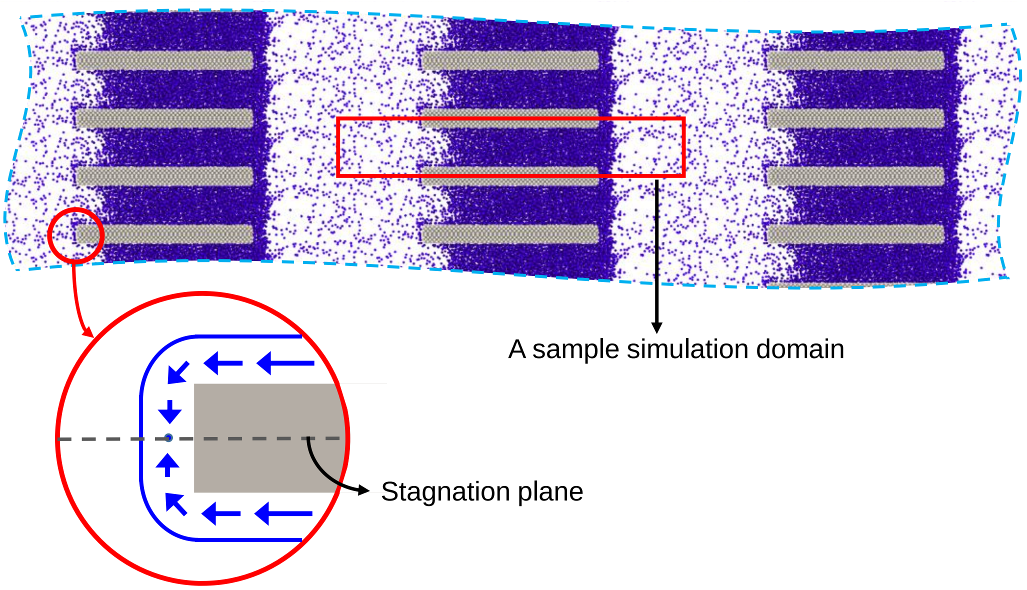


**Figure S3:** A sample simulation domain and its neighboring periodic images.

## S9. Evaporation area selection

The simplest and most common way is to take the cross sectional area of the conduit as the evaporation area (Figure S4a). However, extended evaporating meniscus has larger surface area than cross sectional area, except in extremely small systems, where the adsorbed layer thickness is comparable with the system size. Therefore, this selection usually leads to an overestimation of heat fluxes. Second option is to take the extended meniscus area as the evaporation area (Figure S4b). Surface area of the meniscus extended between the adsorbed layers on the channel walls is calculated based on a curve fit (shown by solid blue line) to the liquid/vapor interface (shown by semi-transparent blue line). Estimated extended meniscus area is slightly smaller than the cross sectional area due to omission of the adsorbed layer. Another option is to take **l**iquid/vapor interfacial area including the adsorbed layer interface as the evaporation area (Figure S4c). Interfacial area of adsorbed layers on both channel walls is added to the extended meniscus area.

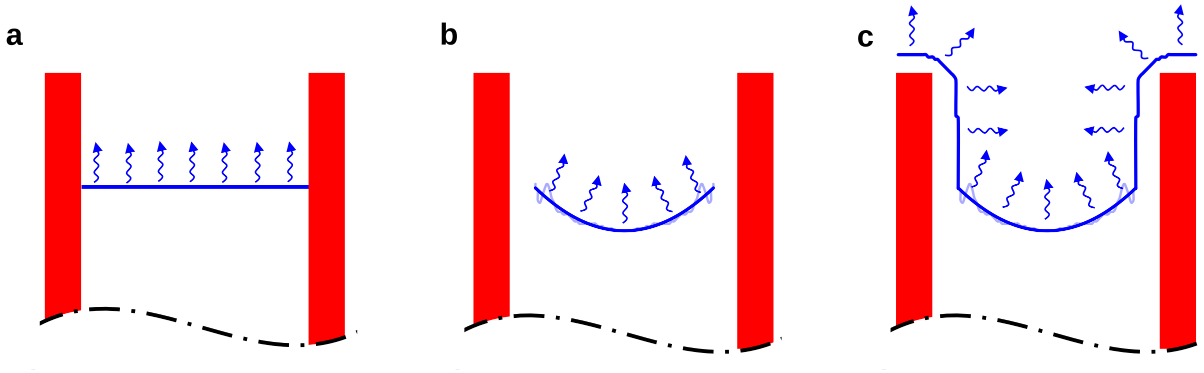


**Figure S4:** Evaporation area selection. **a,** The cross sectional area between channel walls. **b,** Extended meniscus area. **c,** Liquid/vapor interfacial area including the adsorbed layer interface.

## S10. Supplementary Video

Lateral momentum transport within and evaporation from the adsorbed layer is demonstrated by emphasizing the motion of an individual fluid atom in the adsorbed layer.

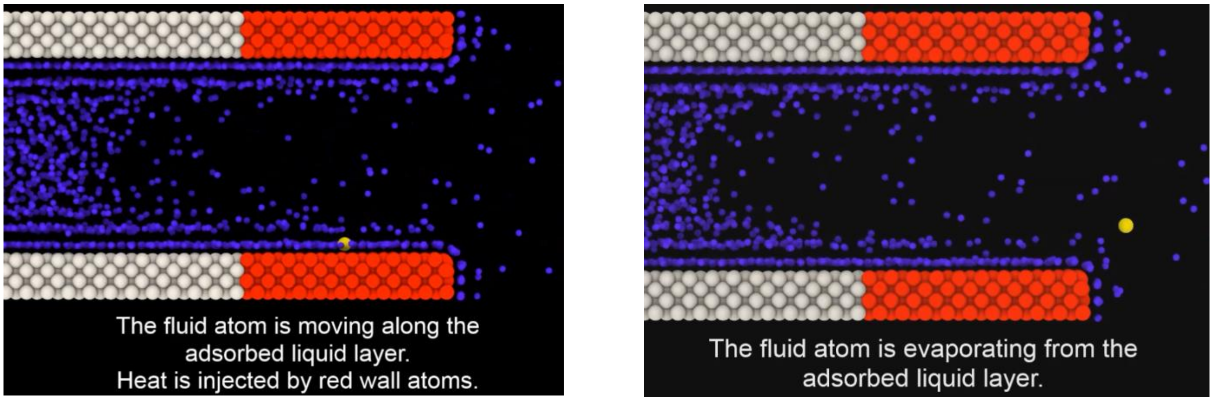


**Figure S5:** Two captions from Supplementary Video
